# Supplementary material for: adcc: A versatile toolkit for rapid development of algebraic-diagrammatic construction methods
Source: arXiv:1910.07757 ancillary file (2019-12-22)
Supplement: Supplementary file 1 [file supporting_info.pdf]

# `adcc`: A versatile toolkit for rapid development of algebraic-diagrammatic construction methods

## Supporting information

Michael F. Herbst, Maximilian Scheurer, Thomas Fransson, Dirk R. Rehn, Andreas Dreuw

## SI-1 Data-based host provider interface

Statically precomputed Hartree-Fock (HF) data can be supplied to `adcc` either as a `python` dictionary or as an HDF5 file [1]. In both cases the dictionary variable or the HDF5 file handle / file name can be passed directly to the ADC method functions of `adcc`. For example, if `data.hdf5` is the file containing the HDF5 HF data to be used in `adcc`, one may run an ADC(2)-x calculation for four singlets as such:

```
adcc.adc2x("data.hdf5", n_singlets=4)
```

Let now `nf` denote the number of Hartree-Fock spin orbitals (i.e., the sum of both the number of alpha and the beta molecular orbitals) and `nb` the number of basis functions. With `array` we indicate either a NumPy array [2] or an HDF5 dataset. The following keys are required in the dictionary or the HDF5 file:

1. **restricted** (`bool`): `True` for a restricted SCF calculation, `False` otherwise
2. **conv_tol** (`float`): Tolerance value used for SCF convergence, should be roughly equivalent to $l_2$-norm of the Pulay error.
3. **orbcoeff_fb** (`array` with `dtype=float`, size `(nf, nb)`): SCF orbital coefficients, i.e., the uniform transform from the basis to the molecular orbitals.
4. **occupation_f** (`array` with `dtype=float`, size `(nf, )`): Occupation number for each SCF orbitals (i.e., diagonal of the HF density matrix in the SCF orbital basis).
5. **orben_f** (`array` with `dtype=float`, size `(nf, )`): SCF orbital energies
6. **fock_ff** (`array` with `dtype=float`, size `(nf, nf)`): Fock matrix in SCF orbital basis. Notice, the full matrix is expected also for restricted calculations.
7. **eri_phys_asym_ffff** (`array` with `dtype=float`, size `(nf, nf, nf, nf)`): Antisymmetrised electron-repulsion integral tensor in the SCF orbital basis, using the Physicists' indexing convention, i.e., that the index tuple `(i,j,k,l)` refers to the integral $\langle ij||kl\rangle$, i.e.,

$$\int_\Omega \int_\Omega dr_1 dr_2 \frac{\phi_i(r_1)\phi_j(r_2)\phi_k(r_1)\phi_l(r_2)}{|r_1 - r_2|} - \int_\Omega \int_\Omega dr_1 dr_2 \frac{\phi_i(r_1)\phi_j(r_2)\phi_l(r_1)\phi_k(r_2)}{|r_1 - r_2|}$$

   The full tensor (including zero blocks) is expected.

As an alternative to eri_phys_asym_ffff, the user may provide

8. **eri_ffff** (`array` with `dtype=float`, size `(nf, nf, nf, nf)`): Electron-repulsion integral tensor in chemists' notation. The index tuple `(i,j,k,l)` thus refers to the integral $(ij|kl)$, which is

$$\int_\Omega \int_\Omega dr_1 dr_2 \frac{\phi_i(r_1)\phi_j(r_1)\phi_k(r_2)\phi_l(r_2)}{|r_1 - r_2|}$$

   Notice, that no antisymmetrisation has been applied in this tensor.

The above keys define the least set of quantities to start a calculation in `adcc`. In order to have access to properties such as dipole moments or to get the correct state energies, further keys are highly recommended to be provided as well.

9. **energy_scf** (`float`): Final total SCF energy of both electronic and nuclear energy terms. (default: 0.0)

10. **multipoles**: Container with electric and nuclear multipole moments. Can be another dictionary or simply an HDF5 group.

    - **elec_1** (`array`, size `(3, nb, nb)`): Electric dipole moment integrals in the atomic orbital basis (i.e., the discretisation basis with `nb` elements). First axis indicates cartesian component (x, y, z).
    - **nuc_0** (`float`): Total nuclear charge
    - **nuc_1** (`array` size `(3, )`): Nuclear dipole moment

    The defaults for all entries are all-zero multipoles.

11. **spin_multiplicity** (`int`): The spin multiplicity of the HF ground state described by the data. A value of 0 (for unknown) should be supplied for unrestricted calculations. (default: 1 for restricted and 0 for unrestricted calculations)

A descriptive string for the backend can be supplied optionally as well. In case of using a python dict as the data container, this should be done using the key backend. For an HDF5 file, this should be done using the attribute backend. Defaults based on the filename are generated. More details and further examples can also be found on our website under `https://adc-connect.org/q/hostprograms`.

# SI-2 Host-program specific interface

For implementing a host-program specific interface to `adcc`, taking advantage of all features of the host program, a derived class of the `adcc.HartreeFockProvider` has to be implemented. The file `HartreeFockProvider.py` shows stub code describing the interface of this class.

# SI-3 Hardware and compiler details

The memory trace and timings for the noradrenaline calculation were carried out on Red Hat Enterprise Linux (RHEL), version 7.5, using the kernel version 3.10.0-862.3.3.el7.x86_64. Openblas 0.3.3, Python 3.7.0, and `adcc` were compiled with the GNU Compiler Collection (gcc) 8.2.0. The `glibc` version was 2.17, whereas `libstdc++` version 6.0.25 was employed. The job ran on four Intel Xeon E5-4620v3 (Haswell) processors, employing 32 processor cores.

## SI-4 Details for reproducing the figures of the paper

For reproducing the figures shown in the main text, the following `python` scripts are enclosed. For our computations we used `adcc` version `0.13.1`.

- `dump_matrices.py` and `plot_matrices.py` to reproduce the ADC matrix plots of Figure 1.
- `procmem_memory.py`, `plot_memory_trace.py` and `pyscf_adc2_noradrenaline.py` are needed to reproduce the memory and time profile of Figure 3.
- `cascade.py` and `plot_cascade.py` can be used to reproduce the *Comparison of ADC methods* example.
- `cvs_example.py` can be used to reproduce the *Flexible selection of frozen MOs and CVS spaces* example.
- The folder `nr_calculations` contains all scripts to reproduce the nile red example, together with employed embedding parameters (`*.pot` files).
  - nile red in vacuum: `vacuum/nile_red_pe_adc2_adcc.py`
  - nile red in water: `water/nile_red_pe_adc2_adcc.py`
  - nile red in BLG: `BLG/nile_red_pe_adc2_adcc.py`

## SI-5 `adcc` timings for selected systems

Table SI-1 displays timings for two molecular systems, Noradrenaline and *p*-Nitroaniline, comparing `adcc` and Q-Chem. For all calculations the same cluster node was employed (2 x Intel Xeon E5-2630 v4 @ 2.20GHz).

For the `adcc` calculation we used version 0.13.3 [3] using the SCF from `pyscf` version 1.6.5. Both packages were installed using `pip` as binaries linked against OpenBLAS version 0.3.3. For the Q-Chem calculation version 5.2 was used, compiled against Intel's Math-Kernel Library version 11.3.2.

For each calculation we requested 7 singlet excited states and used a parallelisation over 20 threads. Default settings were used in `adcc` for the convergence, whereas for Q-Chem the maximum subspace size for the Davidson procedure was explicitly set to 70 to improve convergence. Otherwise defaults were chosen as well, amounting to a convergence threshold of $10^{-6}$ in both packages. All states converged unless indicated otherwise.

Table SI-1: Timings for selected ADC calculations comparing `adcc` and Q-Chem

| | | | Time [s] | |
|---|---|---|---|---|
| System | Method | Basis Set | `pyscf` / `adcc` | Q-Chem 5.2 |
| Noradrenaline | ADC(1) | 6-311++G** | 317 | 413 |
| | ADC(2) | 6-311++G** | 10462 | 11390 a) |
| *p*-Nitroaniline | ADC(1) | cc-pVDZ | 37 | 80 |
| | ADC(2) | cc-pVDZ | 790 | 1389 b) |

a) Only 5 states converged.
b) Only 6 states converged.

## References

[1] *HDF5 Reference Manual*. The HDF Group (2011). Release 1.8.8.

[2] S. van der Walt, S. C. Colbert and G. Varoquaux. *The NumPy Array: A Structure for Efficient Numerical Computation*. Comp. Sci. Eng., **13**, 22 (2011).

[3] M. F. Herbst and M. Scheurer. *adcc v0.13.3* (2019). DOI 10.5281/zenodo.3590027.
